# Supplementary material for: Incommensurate spin fluctuations and competing pairing symmetries in La$_3$Ni$_2$O$_7$
Source: arXiv:2501.05254 source file (2025-11-22)
Supplement: Supplementary file 1 [file supplement.pdf]

# Incommensurate spin fluctuations and competing pairing symmetries in $La_3Ni_2O_7$ – Supplemental Material –

Han-Xiang Xu[1] and Daniel Guterding[2]

[1] *Beijing National Laboratory for Condensed Matter Physics, Institute of Physics, Chinese Academy of Sciences, Beijing 100190, China*

[2] *Technische Hochschule Brandenburg, Magdeburger Straße 50, 14770 Brandenburg an der Havel, Germany*

(Dated: November 22, 2025)

## I. ADDITIONAL ELECTRONIC STRUCTURE RESULTS

In addition to the electronic structure, which we have discussed in the main text, we show here also the three-dimensional Fermi surface (see Fig. S1), the evolution of electronic structure as a function of pressure (see Fig. S2), and the two-dimensional Fermi surface with contribution of orbital characters (see Fig. S3) calculated using density functional theory (DFT).

Fig. S1 shows how the Fermi surface consists of three cylinders with different degree of warping in the $k_z$-direction. The $\alpha$ and $\beta$ Fermi surfaces can be considered almost two-dimensional, but the $\gamma$ Fermi surface is obviously $k_z$ dependent, which is the reason why we discuss the nesting vectors beyond first Brillouin zone in the main text. This is also visible in the pressure evolution of the electronic band structure and Fermi surface in the $k_x$-$k_y$-plane (see Fig. S2). In the band structure we can also see the effects of pressure, which resemble direct changes to the crystal field splitting as discussed in Ref. [1]. Pressure also introduces a minor shrinkage of the hole pockets labeled $\gamma$ around the $X$-point, but otherwise does not lead to any dramatic changes in the electronic structure.

The orbital weights of the most relevant orbitals on the Fermi surface calculated from DFT are shown in Fig. S3. Apparently, the $\alpha$ and $\beta$ Fermi surfaces mostly carry Ni $3d_{x^2-y^2}$ and O1 $2p_x$ / $2p_y$ weight, with minor contributions from Ni $3d_{z^2}$ states. The $\gamma$ Fermi surface carries Ni $3d_{z^2}$ and O2 $2p_z$ weight. Differences between $k_z = 0$ and $k_z = \pi$ are again present, but small in size.

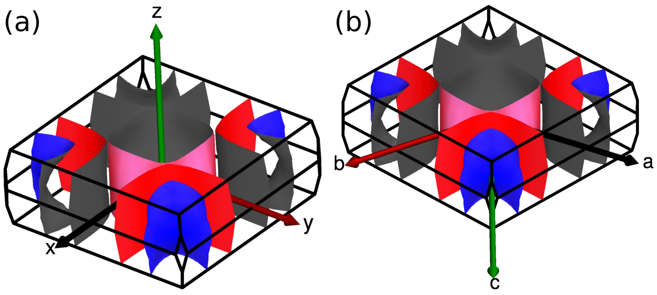


FIG. S1. Three-dimensional Fermi surface in the first Brillouin zone of $La_3Ni_2O_7$ at $P = 24.6$ GPa calculated from DFT. (a) with axes of Cartesian coordinates and (b) with primitive reciprocal lattice vectors.

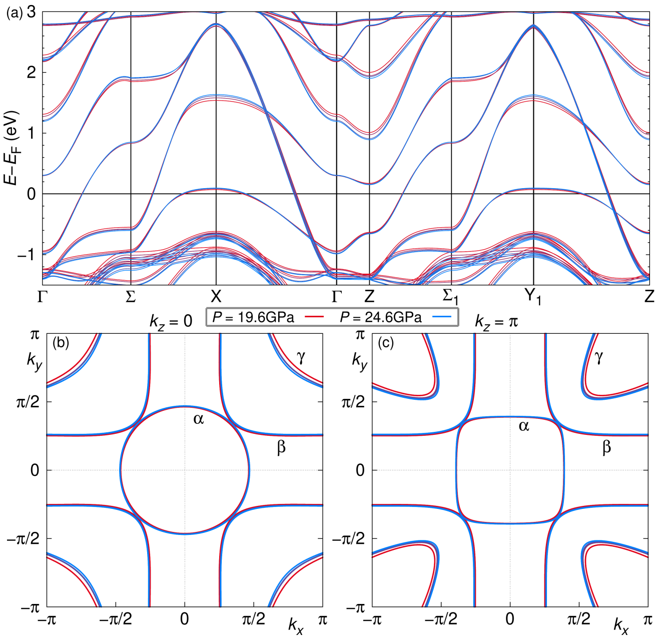


FIG. S2. Pressure evolution of (a) electronic band structure and Fermi surface in the $k_x$-$k_y$-plane at (b) $k_z = 0$ and (c) $k_z = \pi$ calculated from DFT.

## II. TIGHT-BINDING MODEL

We use projective Wannier functions implemented within FPLO [2] to construct accurate tight-binding models for $La_3Ni_2O_7$. The kinetic Hamiltonian is given by:

$$H_0 = -\sum_{i,j} t_{ij}^{sp} c_{is\sigma}^\dagger c_{jp\sigma} \,. \tag{S1}$$

Here, the $t_{ij}^{sp}$ are transfer integrals between sites $i$ and $j$, $s$ and $p$ are orbital indices, and $\sigma$ is the spin.

As can be seen in Fig. S4 (a-d), the quality of agreement for the band structure, density of states and Fermi surface of $La_3Ni_2O_7$ is nearly perfect. To achieve this, we need to include 31 orbitals: ten Ni $3d$ orbitals and twenty-one O $2p$ orbitals.

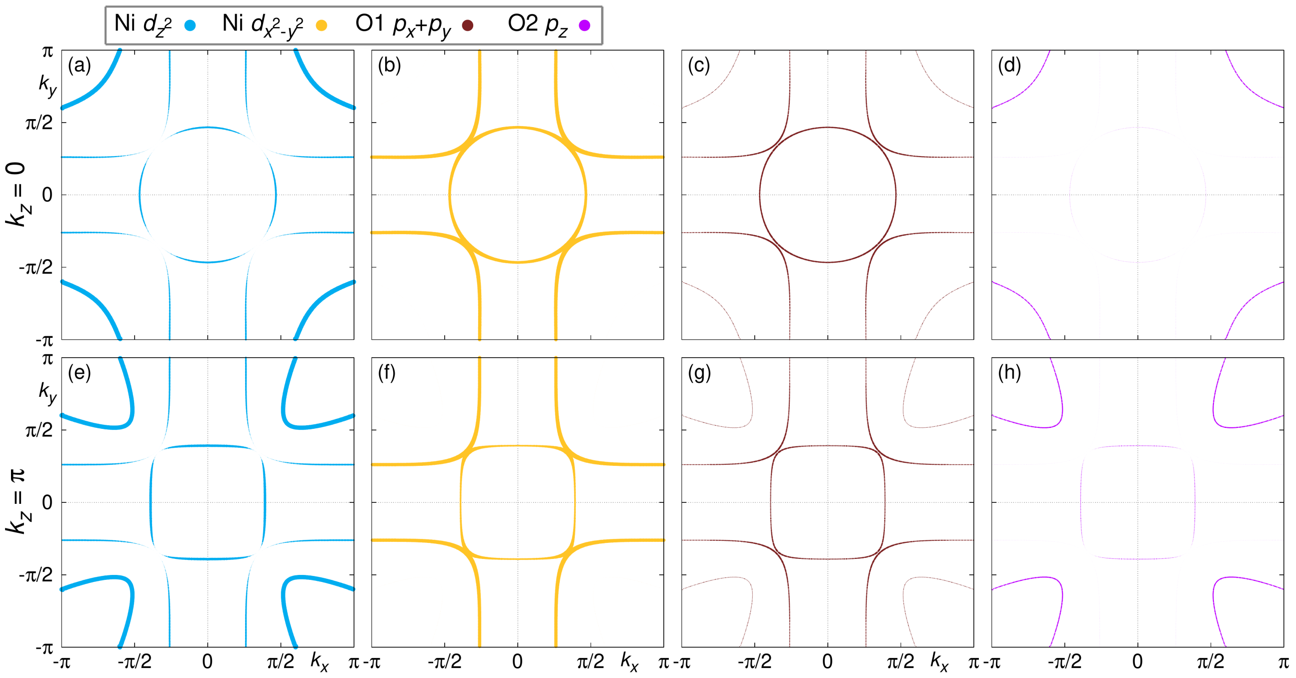


FIG. S3. Orbital weights on the Fermi surface within the $k_x$-$k_y$-plane of $La_3Ni_2O_7$ at $P = 24.6$ GPa calculated from DFT. The top row (a-d) shows the Fermi surface at $k_z = 0$, while the bottom row (e-h) shows $k_z = \pi$.

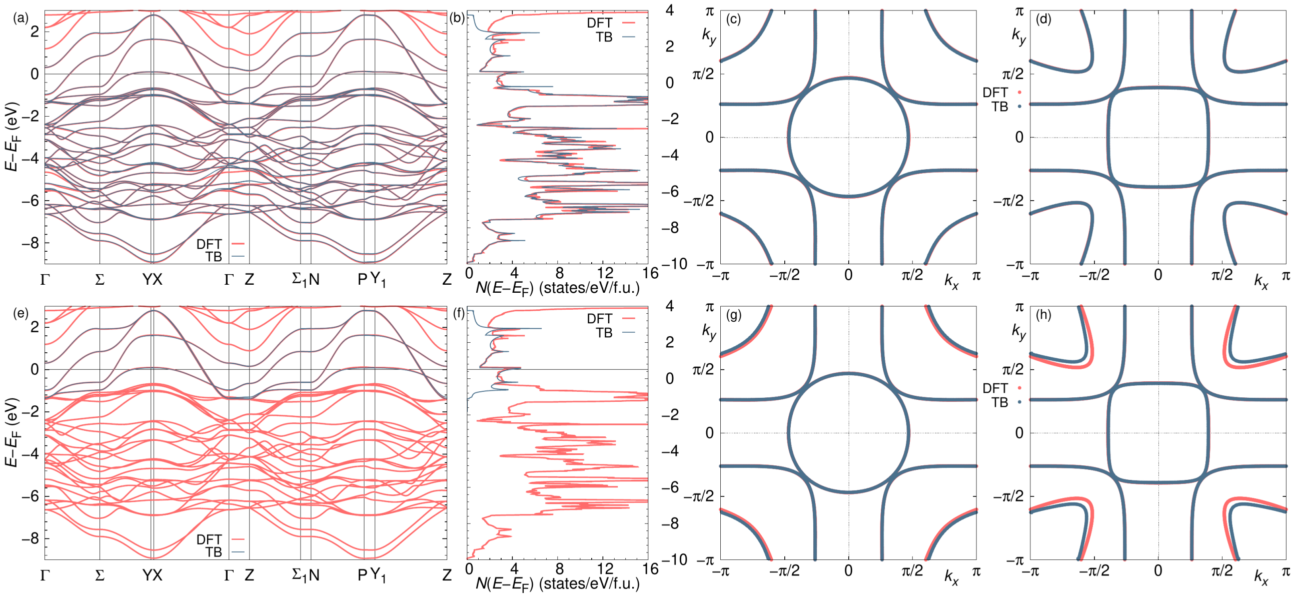


FIG. S4. Comparison between density functional theory and tight-binding model results for $La_3Ni_2O_7$ at $P = 24.6$ GPa. The top row (a-d) shows results for the 31 band model, while the bottom row (e-h) shows the 4 band model. Both models yield a reasonable approximation of the band energies close to the Fermi energy and hence also the total density of states as well as the location of the Fermi surface compared to the full DFT calculation.

## III. COMPARISON BETWEEN 31 BAND AND 4 BAND TIGHT-BINDING MODELS

Previous works for $La_3Ni_2O_7$ have used a 4 band model, which at first glance reproduces the electronic structure close to the Fermi level with high fidelity. Both the Fermi surface and the total density of states are in good agreement with DFT (see Fig. S4 (e-h)). Close to the Fermi level, the four-band model leads to some discrepancies in the band energies w.r.t the DFT results and the 31 band model (see Fig. S5).

Moreover, multi-orbital RPA and also other methods

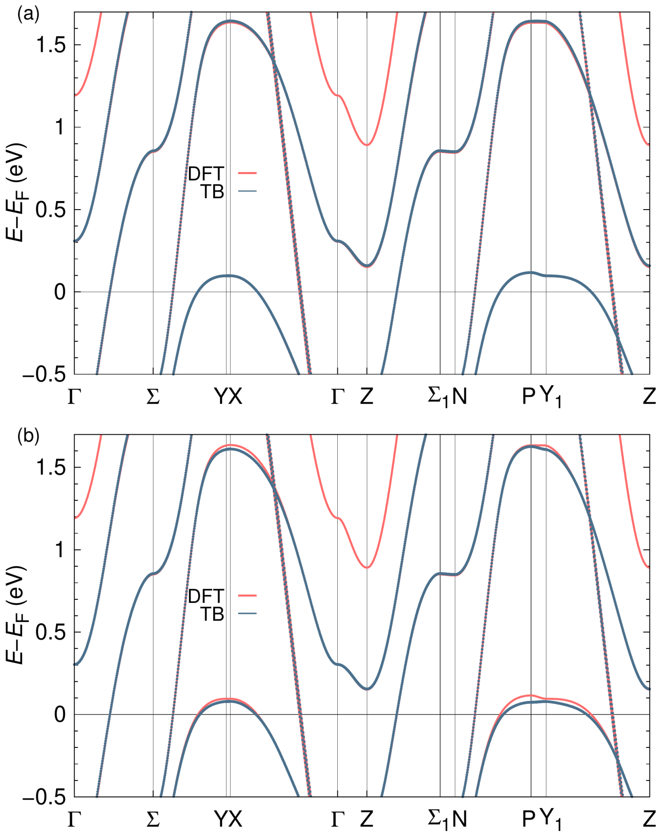


FIG. S5. Comparison between density functional theory (DFT) and tight binding (TB) models for the electronic band structure of $La_3Ni_2O_7$ at $P = 24.6$ GPa. (a) shows the 31 band TB model. (b) shows the 4 band TB model.

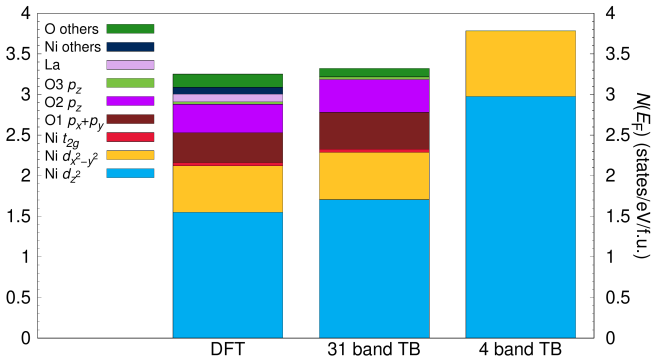


FIG. S6. Histogram of the orbital-resolved density of states at the Fermi level for DFT results, 31 band TB model and 4 band TB model at $P = 24.6$ GPa.

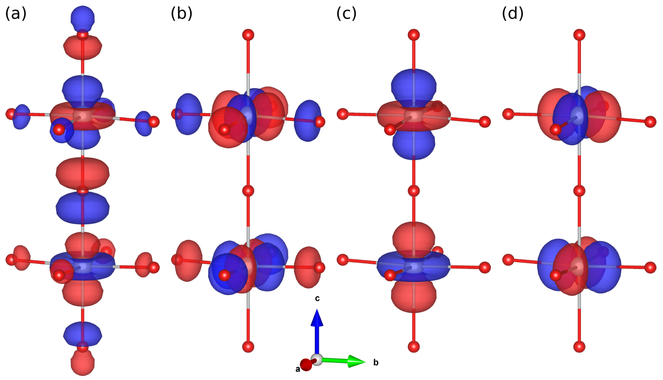


FIG. S7. Wannier functions of the 4 band model for (a) the Ni $3d_{z^2}$ orbital and (b) the Ni $3d_{x^2-y^2}$ orbital. The other two panels show the respective Wannier functions of the 31 band model for (c) the Ni $3d_{z^2}$ orbital and (d) the Ni $3d_{x^2-y^2}$ orbital. The oxygen atoms are shown in red, while the nickel atom in the center of the $NiO_6$ octahedra is shown in grey.

like FLEX or FRG are very sensitive to the orbital matrix elements on the Fermi surface. We believe that the disagreement between seemingly similar models and methods that is evident in the literature can be explained to some degree by the usage of too small models like the previously mentioned 4 band model. To this end, we prepared a histogram of the orbital-resolved contributions to the total density of states at the Fermi level (see Fig. S6). Obviously, the orbital-resolved contributions within the 31 band model are very close to the DFT calculation, while the 4 band model shows a massive overestimation of the Ni $3d_{z^2}$, and to a smaller degree of Ni $3d_{x^2-y^2}$ weights. In DFT the Ni $3d_{z^2}$ and Ni $3d_{x^2-y^2}$ weights are spread over a large energy range because of the strong hybridization with oxygen states. In the 4 band TB model, all Ni $3d_{z^2}$ and Ni $3d_{x^2-y^2}$ states are compressed into the small energy window of the TB model, and replace all the other states which contribute to this energy window in DFT.

A similar effect can also be observed for the Wannier functions of Ni $3d_{z^2}$ and Ni $3d_{x^2-y^2}$ orbitals in the 4 band model (see Fig. S7 (a) and (b)). These are very delocalized and have significant weight on the surrounding oxygen atoms. In contrast, the 31 band model leads to localized atomic-like Wannier functions centered on the Ni atoms (see Fig. S7 (c) and (d)).

This overestimation of nickel weights on the Fermi surface, together with the delocalized Wannier functions, explains why the RPA instability in the 4 band model appears at unrealistically small values for the interaction parameters. The redistribution of orbital weights, however, does not only appear as a function of energy, but also as a function of momentum. From Fig. S3 it is clear that replacing O1 and O2 weights by Ni $3d_{z^2}$ and Ni $3d_{x^2-y^2}$ weights will lead to a strongly altered distribution of orbital weights on the Fermi surface and hence distort the results of any low-energy theory of superconductivity in $La_3Ni_2O_7$, calculated from whatever theoretical method. We believe that this issue is the key to understanding the wide variety of contradictory results reported for $La_3Ni_2O_7$.

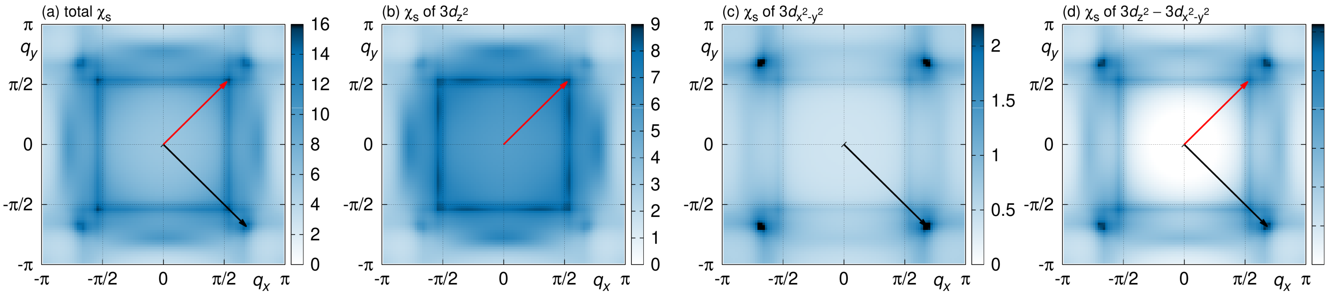


FIG. S8. RPA interacting spin susceptibilities of $La_3Ni_2O_7$ for (a) total $\chi_s$, (b) $(\chi_s)^{qq}_{qq}$, (c) $(\chi_s)^{pp}_{pp}$, and (d) $(\chi_s)^{qq}_{pp}$, where $U = 3$ eV and $J = 0.75$ eV at $P = 24.6$ GPa (with abbreviations $p = d_{x^2-y^2}$ and $q = d_{z^2}$).

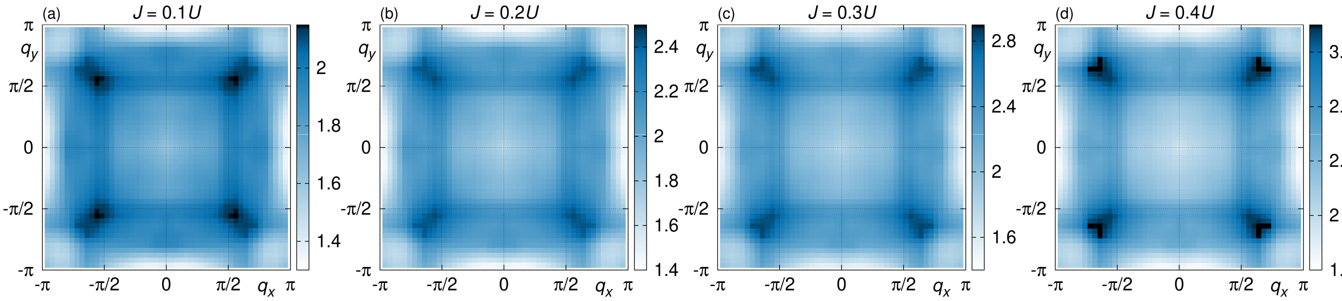


FIG. S9. Evolution of RPA interacting spin susceptibilities for $P = 24.6$ GPa at $U = 2.5$ eV with increasing Hund's rule coupling $J$.

## IV. SPIN FLUCTUATION FORMALISM

We consider the multiorbital Hubbard Hamiltonian [3]:

$$\begin{aligned} H =& H_0 + U\sum_{i,l} n_{il\uparrow}n_{il\downarrow} + \frac{U'}{2}\sum_{i,s,p\neq s} n_{is}n_{ip} \\ &- \frac{J}{2}\sum_{i,s,p\neq s} \boldsymbol{S}_{is}\cdot\boldsymbol{S}_{ip} + \frac{J'}{2}\sum_{i,s,p\neq s,\sigma} c^\dagger_{is\sigma}c^\dagger_{is\bar\sigma}c_{ip\bar\sigma}c_{ip\sigma}\,, \end{aligned} \tag{S2}$$

with Fermionic creation (annihilation) operators $c^\dagger_{is\sigma}$ ($c_{is\sigma}$), spin operator $\boldsymbol{S}_{is}$, density operator $n_{is\sigma} = c^\dagger_{is\sigma}c_{is\sigma}$ and interaction parameters $U$ (intra-orbital Coulomb repulsion), $U'$ (inter-orbital Coulomb repulsion), $J$ (Hund's rule coupling) and $J'$ (pair-hopping term).

The tight binding part $H_0$ is given by Eq. (S1). Diagonalization of $H_0$ provides band energies $E_l(\boldsymbol{k})$ and matrix elements $a^t_l$ and enables us to calculate the static non-interacting susceptibility:

$$\begin{aligned} \chi^{pq}_{st}(\boldsymbol{q}) =& -\sum_{\boldsymbol{k},l,m} a^{p*}_l(\boldsymbol{k})a^t_l(\boldsymbol{k})a^{s*}_m(\boldsymbol{k}+\boldsymbol{q})a^q_m(\boldsymbol{k}+\boldsymbol{q}) \\ &\times \frac{n_F(E_l(\boldsymbol{k})) - n_F(E_m(\boldsymbol{k}+\boldsymbol{q}))}{E_l(\boldsymbol{k}) - E_m(\boldsymbol{k}+\boldsymbol{q})}\,, \end{aligned} \tag{S3}$$

where $n_F(E)$ is the Fermi-Dirac distribution function. We use an inverse temperature of $\beta = (k_BT)^{-1} = 40\,\text{eV}^{-1}$ for the susceptibility calculation. The observable static susceptibility can be calculated as:

$$\chi_0(\boldsymbol{q}) = \frac{1}{2}\sum_{ab}\chi^{bb}_{aa}(\boldsymbol{q})\,. \tag{S4}$$

Applying the multi-orbital random phase approximation (RPA) [3, 4], charge and spin susceptibilities are calculated from the non-interacting susceptibility as:

$$\begin{aligned} \left[(\chi^{RPA}_{\mathrm{c}})^{pq}_{st}\right]^{-1} &= \left[\chi^{pq}_{st}\right]^{-1} + (U_{\mathrm{c}})^{pq}_{st} \\ \left[(\chi^{RPA}_{\mathrm{s}})^{pq}_{st}\right]^{-1} &= \left[\chi^{pq}_{st}\right]^{-1} - (U_{\mathrm{s}})^{pq}_{st}\,, \end{aligned} \tag{S5}$$

where nonzero components of the multi-orbital Hubbard model interaction tensors [3] are given by:

$$\begin{aligned} (U_{\mathrm{c}})^{aa}_{aa} &= U\,, & (U_{\mathrm{c}})^{aa}_{bb} &= 2U'\,, \\ (U_{\mathrm{c}})^{ab}_{ab} &= \frac{3}{4}J - U'\,, & (U_{\mathrm{c}})^{ba}_{ab} &= J'\,, \\ (U_{\mathrm{s}})^{aa}_{aa} &= U\,, & (U_{\mathrm{s}})^{aa}_{bb} &= \frac{1}{2}J\,, \\ (U_{\mathrm{s}})^{ab}_{ab} &= \frac{1}{4}J + U'\,, & (U_{\mathrm{s}})^{ba}_{ab} &= J'\,. \end{aligned} \tag{S6}$$

Using this approximation for the interacting susceptbilities $\chi^{RPA}_{c/s}$, the superconducting pairing vertex in the singlet channel [3] can be written as:

$$\begin{aligned} \Gamma^{pq}_{st}(\mathbf{k},\mathbf{k}') =& \Bigg[\frac{3}{2}U_s\,\chi^{RPA}_s(\mathbf{k}-\mathbf{k}')\,U_s + \frac{1}{2}U_s \\ &- \frac{1}{2}U_c\,\chi^{RPA}_c(\mathbf{k}-\mathbf{k}')U_c + \frac{1}{2}U_c\Bigg]^{tq}_{ps}\,. \end{aligned} \tag{S7}$$

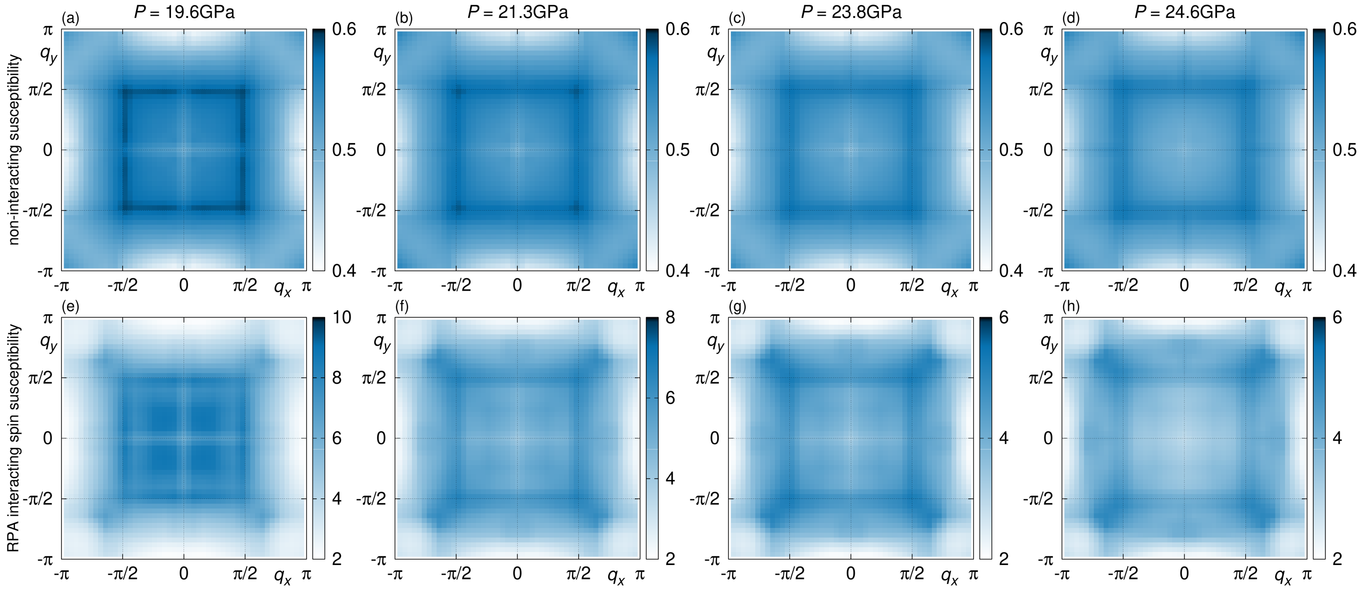


FIG. S10. Pressure evolution of non-interacting susceptibilities (a-d) and RPA interacting spin susceptibilities at $U = 2.8$ eV, $J = 0.7$ eV (e-h).

This vertex in orbital space is projected onto band space using the matrix elements $a_l^t$ of the kinetic Hamiltonian $H_0$:

$$\Gamma_{ij}(\mathbf{k},\mathbf{k}') = \sum_{s,t,p,q} a_i^{t*}(-\mathbf{k}) a_i^{s*}(\mathbf{k}) \mathrm{Re}\left[\Gamma_{st}^{pq}(\mathbf{k},\mathbf{k}')\right] a_j^p(\mathbf{k}') a_j^q(-\mathbf{k}'). \tag{S8}$$

The linearized Eliashberg equation with band-projected pairing vertex $\Gamma_{ij}$ [3] then reads:

$$-\sum_j \oint_{C_j} \frac{dk'_\parallel}{2\pi} \frac{1}{4\pi v_F(\mathbf{k}')} \left[\Gamma_{ij}(\mathbf{k},\mathbf{k}') + \Gamma_{ij}(\mathbf{k},-\mathbf{k}')\right] g_j(\mathbf{k}') = \lambda_i g_i(\mathbf{k})\,. \tag{S9}$$

This equation is solved for the pairing eigenvalue $\lambda_i$ and the gap function on the Fermi surface $g_i(\mathbf{k})$.

## V. ADDITIONAL SUSCEPTIBILITY RESULTS

In addition to the results shown in the main text, we show the orbital-resolved RPA interacting susceptibilities (see Fig. S8), the evolution of RPA interacting susceptibilities with increasing Hund's rule coupling $J$ (see Fig. S9), and the pressure evolution of both non-interacting and RPA interacting spin susceptibilities (see Fig. S10).

Fig. S8 (a) is identical to Fig. 2 (b) in the main text. Fig. S8 (b), (c), and (d) show the contributions of orbital-resolved susceptibilities for the intra-orbital $3d_{z^2}$, intra-orbital $3d_{x^2-y^2}$, and inter-orbital $3d_{z^2} - 3d_{x^2-y^2}$ (off-diagonal element) separately. By analyzing the susceptibility peaks, we can find that the peak at $\mathbf{q}_1 \sim (\pi/2, \pi/2)$ is the highest peak mainly contributed by the spin susceptibility of intra-orbital $3d_{z^2}$, and $\mathbf{q}_2 \sim (7\pi/10, 7\pi/10)$ is the highest peak mainly contributed by intra-orbital $3d_{x^2-y^2}$. Naturally, the spin susceptibility of inter-orbital $3d_{z^2}$-$3d_{x^2-y^2}$ contributes to both $\mathbf{q}_1 \sim (\pi/2, \pi/2)$ and $\mathbf{q}_2 \sim (7\pi/10, 7\pi/10)$ peaks.

Fig. S9 shows that increasing Hund's rule coupling (and indirectly also pair hopping $J'$) switches the dominant peak in the spin susceptibility from $\mathbf{q}_1 \sim (\pi/2, \pi/2)$ to $\mathbf{q}_2 \sim (7\pi/10, 7\pi/10)$. Together with the results from Fig. S8 it is clear that the Hund's rule coupling enhances inter-orbital contributions to the spin susceptibility, which also contribute to the peak at $\mathbf{q}_2 \sim (7\pi/10, 7\pi/10)$. This bears some similarity to the bilayer Hubbard model physics discussed in Ref. [5], although the electronic structure in that study differs from ours in possibly relevant details.

Fig. S10 shows the pressure evolution of susceptibilities. For non-interacting susceptibilities (see Fig. S10 (a-d)), we observe the maximum intensity of the susceptibility peak at low pressure, close to the boundary of the RPA instability. The values of RPA interacting spin susceptibilities (see Fig. S10 (e-h)) clearly decrease with increasing pressure. Moreover, at low pressure (Fig. S10 (e)) we find that several humps appear close to the Brillouin zone center Γ. This shows how the susceptibility diverges when the system is close to the RPA instability, which we demonstrated is the case near the low-pressure region of the $I4/mmm$ phase of $La_3Ni_2O_7$.

Therefore, it seems that $La_3Ni_2O_7$ under pressure is close to a magnetic instability. The ordering tendency is not strong enough to realize a long-range ordered state,

and is further suppressed, together with a slight reduction of the superconducting transition temperature, as pressure is applied.


[1] C. Xia, H. Liu, S. Zhou, and H. Chen, Sensitive dependence of pairing symmetry on Ni-$e_g$ crystal field splitting in the nickelate superconductor $La_3Ni_2O_7$, Nat. Commun. **16**, 1054 (2025).

[2] H. Eschrig and K. Koepernik, Tight-binding models for the iron-based superconductors, Phys. Rev. B **80**, 104503 (2009).

[3] S. Graser, T. A. Maier, P. J. Hirschfeld, and D. J. Scalapino, Near-degeneracy of several pairing channels in multiorbital models for the Fe pnictides, New J. Phys. **11**, 025016 (2009).

[4] M. Altmeyer, D. Guterding, P. J. Hirschfeld, T. A. Maier, R. Valentí, and D. J. Scalapino, Role of vertex corrections in the matrix formulation of the random phase approximation for the multiorbital Hubbard model, Phys. Rev. B **94**, 214515 (2016).

[5] Y. Nomura, M. Kitatani, S. Sakai, and R. Arita, Strong-coupling high-$T_c$ superconductivity in doped correlated band insulators, Phys. Rev. B **112**, L020504 (2025).
